# Supplementary material for: Latent modeling of flow cytometry cell populations
Source: arXiv:1502.04058 ancillary file (2015-02-13)
Supplement: Supplementary file 1 [file SupplementMat.pdf]

# Latent modeling of flow cytometry cell populations
# — Supplemental Material

Jonas Wallin[1], Kerstin Johnsson*[2], and Magnus Fontes[2,3]

[1]Mathematical Sciences, Chalmers and University of Gothenburg
[2]Centre for Mathematical Sciences, Lund University
[3]Institut Pasteur, Paris

February 13, 2015

*johnsson@maths.lth.se; Corresponding author

# A Posterior

The posterior distribution given the model (1), (2), the priors (3) and data $\mathbf{Y}$ is

$$\pi(\boldsymbol{\Theta}|\mathbf{Y},\mathbf{x})$$
$$\propto \left(\prod_{j=1}^{J}\prod_{i=1}^{n_j}|\boldsymbol{\Sigma}_{j\mathbf{x}_{ij}}|^{-1/2}\exp\left(-\frac{1}{2}(\mathbf{Y}_{ij}-\boldsymbol{\mu}_{j\mathbf{x}_{ij}})^\top\boldsymbol{\Sigma}_{j\mathbf{x}_{ij}}^{-1}(\mathbf{Y}_{ij}-\boldsymbol{\mu}_{j\mathbf{x}_{ij}})\right)\pi_{j\mathbf{x}_{ij}}\right)\cdot$$
$$\left(\prod_{j=1}^{J}\prod_{k=1}^{K}\pi_{jk}^{a_{jk}}|\boldsymbol{\Sigma}_{\theta_k}|^{-\frac{1}{2}}\exp\left(-\frac{1}{2}(\boldsymbol{\mu}_{jk}-\boldsymbol{\theta}_k)^\top\boldsymbol{\Sigma}_{\theta_k}^{-1}(\boldsymbol{\mu}_{jk}-\boldsymbol{\theta}_k)\right)\right.$$
$$\left.\frac{|\boldsymbol{\Sigma}_{jk}|^{-\frac{\nu_k+d+1}{2}}|\boldsymbol{\Psi}_k|^{\frac{\nu_k}{2}}}{2^{\frac{\nu_k d}{2}}\Gamma_d(\frac{\nu_k}{2})}\exp\left(-\mathrm{tr}(\boldsymbol{\Psi}_k\boldsymbol{\Sigma}_{jk}^{-1})/2\right)\right)\cdot$$
$$\left(\prod_{k=1}^{K}\exp\left(-\frac{1}{2}(\boldsymbol{\theta}_k-\mathbf{t}_k)^\top\mathbf{S}_k^{-1}(\boldsymbol{\theta}_k-\mathbf{t}_k)\right)|\boldsymbol{\Psi}_k|^{\frac{n_\Psi-d-1}{2}}\exp\left(-\mathrm{tr}(\mathbf{H}_k^{-1}\boldsymbol{\Psi}_k)/2\right)\right.$$
$$\left.|\boldsymbol{\Sigma}_{\theta_k}|^{-\frac{n_\theta}{2}}\exp\left(-\mathrm{tr}(\mathbf{Q}_k\boldsymbol{\Sigma}_{\theta_k}^{-1})/2\right)\exp(-\lambda_k\nu_k)\right). \quad (1)$$

# B Sampling from the posterior distribution

We use a Markov Chain Monte Carlo (MCMC) algorithm to generate samples from the posterior distribution of the parameters (Robert and Casella, 2004). In each iteration we draw a value of each of the parameters $\boldsymbol{\Theta}$ and of $\mathbf{x}$. The backbone of our algorithm is a Gibbs sampler, but we need a Metropolis-Hastings step to sample $\nu_k$. We also use Metropolis-Hastings steps to enable label-switching—which improves the mixing of the Gibbs sampler—and to turn on and off mixture components in the extended model with absent clusters.

In a Gibbs sampler samples from the full posterior distribution is obtained by successively sampling from the conditional posterior distributions of each of the variables given all other variables. First we sample the component assigment variables, $\mathbf{x}$, fixing all other parameters. The posterior from which we sample is a multinomial distribution with

$$\pi(x_{ij}=k|\ldots)\propto\frac{N(\mathbf{Y}_{ij};\boldsymbol{\mu}_{jk},\boldsymbol{\Sigma}_{jk})\pi_{jk}}{\sum_{h=0}^{K}N(\mathbf{Y}_{ij};\boldsymbol{\mu}_{jh},\boldsymbol{\Sigma}_{jh})\pi_{jh}},$$

where '...' denotes conditioning on all parameter except the one of interest.

Let $n_{jk}$ denote the number of $i$ such that $x_{ij} = k$ and let $\mathbf{Y}_{.jk}$ denote the vector joining all $\mathbf{Y}_{ij}$ such that $x_{ij} = k$. The following Gibbs steps that follows are derived from the posterior distribution (1)

$$\begin{aligned}
\boldsymbol{\pi}_j|\ldots &\sim D(a + n_{j1}, \ldots, a + n_{jK}),\\
\boldsymbol{\Sigma}_{jk}|\ldots &\sim IW(\boldsymbol{\Psi}_k + \sum_{i=1}^{n_{jk}} (\mathbf{Y}_{ijk} - \boldsymbol{\mu}_{jk})(\mathbf{Y}_{ijk} - \boldsymbol{\mu}_{jk})^\top, n_{jk} + \nu_k),\\
\boldsymbol{\mu}_{jk}|\ldots &\sim N_C(\boldsymbol{\Sigma}_{\theta_k}^{-1}\boldsymbol{\theta}_k + \boldsymbol{\Sigma}_{jk}^{-1}\sum_{i=1}^{n_{jk}} \mathbf{Y}_{ijk}, \boldsymbol{\Sigma}_{\theta_k}^{-1} + n_{jk}\boldsymbol{\Sigma}_{jk}^{-1}),\\
\boldsymbol{\Sigma}_{\theta_k}|\ldots &\sim IW(\mathbf{Q}_k + \sum_{j=1}^{J} (\boldsymbol{\mu}_{jk} - \boldsymbol{\theta}_k)(\boldsymbol{\mu}_{jk} - \boldsymbol{\theta}_k)^\top, J + n_\theta),\\
\boldsymbol{\Psi}_k|\ldots &\sim W\left(\left(\mathbf{H}_k^{-1} + \sum_{j=1}^{J} \boldsymbol{\Sigma}_{jk}^{-1}\right)^{-1}, n_\Psi + J\nu_k\right),\\
\boldsymbol{\theta}_k|\ldots &\sim N_C(\mathbf{S}_k^{-1}\mathbf{t}_k + \boldsymbol{\Sigma}_{\theta_k}^{-1}\sum_{j=1}^{J} \boldsymbol{\mu}_{jk}, \mathbf{S}_k^{-1} + J\boldsymbol{\Sigma}_{\theta_k}^{-1}).
\end{aligned}$$

Here $N_C$ denotes the canonical parameterization of the normal distribution, which means that if $\mathbf{x} \sim N_C(\mathbf{b}, \mathbf{Q})$, then $\pi(\mathbf{x}) \propto \exp\left(-\frac{1}{2}\mathbf{x}^\top\mathbf{Q}\mathbf{x} + \mathbf{b}^\top\mathbf{x}\right)$.

To handle the non-standard conditional distribution of $\nu_k$, we utilize a Metropolis-Hastings (MH) algorithm. A proposal $\nu_k^*$ is generated by sampling $\nu_k^* \sim \nu_k + Z$, where $Z$ is uniformly distributed on $\{-r, -r+1, \ldots, r\}$ for some $r \in \mathbb{N}^+$. Hence the transition density $q(\nu_k, \nu_k^*) = q(\nu_k|\nu_k^*)$ is constant on its support. The proposed $\nu_k^*$ is accepted with probability

$$\alpha(\nu_k, \nu_k^*) = \min\left(1, \frac{\pi(\nu_k^*)q(\nu_k^*, \nu)}{\pi(\nu_k)q(\nu, \nu_k^*)}\right) = \min\left(1, \frac{\pi(\nu_k^*)}{\pi(\nu_k)}\right),$$

where $\pi(\nu_k)$ denotes the posterior distribution of $\nu_k$ given all other parameters and data. Using (1) we get that

$$\alpha(\nu_k, \nu_k^*) = \min\left(1, \prod_{j=1}^{J} \frac{\Gamma_d(\frac{\nu_k}{2})}{\Gamma_d(\frac{\nu_k^*}{2})} \left(2^d|\boldsymbol{\Sigma}_{jk}||\boldsymbol{\Psi}_k|^{-1}\right)^{\frac{\nu_k - \nu_k^*}{2}} \exp\left(\lambda_k(\nu_k^* - \nu_k)\right)\right).$$

If $\nu_k^*$ is accepted it will be the new sample, otherwise the new sample will be $\nu_k$.

## B.1 Label switching

An issue that frequently occurs, especially with poor starting values, is that a cluster $\{\boldsymbol{\mu}_{jk_1}, \boldsymbol{\Sigma}_{jk_1}, \pi_{jk_1}\}$ is incorrectly assigned to the latent cluster $k_1$ when it clearly should belong to $k_2$. When the number cells is large the first row of (1) will dominate the posterior so that $\{\boldsymbol{\mu}_{jk_1}, \boldsymbol{\Sigma}_{jk_1}, \pi_{jk_1}\}$ or $\{\boldsymbol{\mu}_{jk_2}, \boldsymbol{\Sigma}_{jk_2}, \pi_{jk_2}\}$ does not change much at all in the updating step and thus in practice the clusters will never move close enough to each other in order to switch locations.

To remedy this issue, we introduce an extra MH step where labels can be switched between clusters in each sample $j$ in each iteration. The proposed MH algorithm has a symmetric transition kernel, where two labels $k_1$ and $k_2$ are sampled from $\{1, \ldots, K\}$ with equal probability. The proposed switch is accepted with probability

$$\alpha(k_1, k_2) = \min\left(1, \frac{\pi(\mu_{jk_2}|\boldsymbol{\theta}_{k_1}, \boldsymbol{\Sigma}_{\theta_{k_1}})\pi(\mu_{jk_1}|\boldsymbol{\theta}_{k_2}, \boldsymbol{\Sigma}_{\theta_{k_2}})}{\pi(\mu_{jk_1}|\boldsymbol{\theta}_{k_1}, \boldsymbol{\Sigma}_{\theta_{k_1}})\pi(\mu_{jk_2}|\boldsymbol{\theta}_{k_2}, \boldsymbol{\Sigma}_{\theta_{k_2}})} \frac{\pi(\boldsymbol{\Sigma}_{jk_1}|\boldsymbol{\Psi}_{k_2}, \nu_{k_2})\pi(\boldsymbol{\Sigma}_{jk_2}|\boldsymbol{\Psi}_{k_1}, \nu_{k_1})}{\pi(\boldsymbol{\Sigma}_{jk_1}|\boldsymbol{\Psi}_{k_1}, \nu_{k_1})\pi(\boldsymbol{\Sigma}_{jk_2}|\boldsymbol{\Psi}_{k_2}, \nu_{k_2})}\right). \quad (2)$$

## B.2 Cluster activation and deactivation

In the extended model where components can be absent in some samples we use a reversible jump MH-algorithm (Green, 1995) to enable changes to the dimension of the model. We use the indicator variable $\mathbf{Z}_j$ to keep track of which components that are active; $Z_{jk} = 1$ if component $k$ is active in sample $j$ and $Z_{jk} = 0$ otherwise.

Activation or deactivation is proposed as the last step of each iteration of the MCMC algorithm. Throughout the activation/deactivation step the component assignment variables $x_{ij}$ are integrated out of the posterior.

A deactivation of an active component is proposed with probability $p_d$ and an activation of a component that is not active is proposed with probability $p_a$. The component that is proposed to be deactivated/activated is chosen randomly among the clusters that are active or not active respectively with equal probability. The probability of proposing to deactivate component $k$ in sample $j$ is

$$q(Z_{jk} = 1 \to 0) = \frac{p_d}{\sum_{l=1}^{K} Z_{jl}}.$$

The probability of proposing to activate component $k$ in sample $j$ is

$$q(Z_{jk} = 0 \to 1) = \frac{p_a}{K - \sum_{l=1}^{K} Z_{jl}}.$$

If an activation step is proposed it is necessary to generate parameters for the new component; they are obtained in the following way:

$$\begin{aligned} \pi_{jk}^* &\sim \text{Beta}(\alpha, \beta), \\ \boldsymbol{\mu}_{jk}^* &\sim N(\boldsymbol{\theta}_k, \boldsymbol{\Sigma}_{\theta_k}), \\ \boldsymbol{\Sigma}_{jk}^* &\sim IW(\boldsymbol{\Psi}_k, \nu_k). \end{aligned}$$

Here $\alpha$ and $\beta$ is chosen so that the probability $\pi_{jk}^*$ is typically close to zero. The transition density $q_{k_j}(\boldsymbol{\mu}_{jk}^*, \boldsymbol{\Sigma}_{jk}^*, \pi_{jk}^*)$ is the joint density of these new parameters when they are sampled as above. For the remaining components we keep the mean and covariance parameters, $\boldsymbol{\mu}_{jl}^* = \boldsymbol{\mu}_{jl}$ and $\boldsymbol{\Sigma}_{jl}^* = \boldsymbol{\Sigma}_{jl}$ for $l \neq k$, but the probabilities $\boldsymbol{\pi}_j$ have to be modified. In the reversible jump algorithm this is done in a dimension matching transform. When activating a cluster we set $\pi_{jl}^* = (1 - \pi_{jk}^*)\pi_{jl}$ for $l \neq k$ in the transform and when deactivating a cluster we set $\pi_{jl}^* = \pi_{jl}/(1 - \pi_{jk})$ for $l \neq k$.

In order to make the Markov chain reversible it is necessary to add the Jacobian of the variable change in the dimension matching transform as a factor in the acceptance probability. Let $\boldsymbol{\Theta}^*$ denote the set of parameters in the proposed model and let $\boldsymbol{\Theta}$ denote the set of current parameters. In an activation step we get (Richardson and Green, 1997)

$$\left| \frac{\partial(\boldsymbol{\Theta}^*)}{\partial\left(\boldsymbol{\Theta}, \pi_{jk}^*, \boldsymbol{\mu}_{jk}^*, \boldsymbol{\Sigma}_{jk}^*\right)} \right| = (1 - \pi_{jk}^*)^{\sum_{l=1}^{K} Z_{jl}},$$

and in a deactivation step the Jacobian is the inverse.

We are now ready to define the acceptance probability for a proposed $\boldsymbol{\Theta}^*$ which implies activation of component $k$ in sample $j$. The acceptance probability equals

$$\alpha\left(\boldsymbol{\Theta}, \boldsymbol{\Theta}^*\right) = \min\left\{1, \frac{\pi(\boldsymbol{\Theta}^*|\mathbf{Y})q(Z_{jk} = 1 \to 0)}{\pi(\boldsymbol{\Theta}|\mathbf{Y})q_{k_j}(\boldsymbol{\mu}_{jk}^*, \boldsymbol{\Sigma}_{jk}^*, \pi_{jk}^*)q(Z_{jk}^* = 0 \to 1)} \left| \frac{\partial(\boldsymbol{\Theta}^*)}{\partial\left(\boldsymbol{\Theta}, \pi_{jk}^*, \boldsymbol{\mu}_{jk}^*, \boldsymbol{\Sigma}_{jk}^*\right)} \right| \right\}, \quad (3)$$

where $\pi(\mathbf{\Theta}^*|\mathbf{Y})$ is the posterior distribution (1) with $x_{ij}$ integrated out. This can be written as

$$\alpha\left(\mathbf{\Theta},\, \mathbf{\Theta}^*\right) = \min\left\{1, \frac{\prod_{i=1}^{n_j}\sum_{l=1}^{K} Z_{jl}^*\pi_{jl}^* N(\mathbf{Y}_{ij}; \boldsymbol{\mu}_{jl}^*, \mathbf{\Sigma}_{jl}^*)}{\prod_{i=1}^{n_j}\sum_{l=1}^{K} Z_{jl}\pi_{jl} N(\mathbf{Y}_{ij}; \boldsymbol{\mu}_{jl}, \mathbf{\Sigma}_{jl})} \cdot \right.$$
$$\left. \frac{D(\boldsymbol{\pi}_j^*; \mathbf{a})\exp(-c_s)}{\mathrm{Beta}(\pi_{jk}^*; \alpha, \beta) D(\mathbf{p}_j; \mathbf{a})} \frac{\frac{p_d}{\sum_{l=1}^{K} Z_{jl}}}{\frac{p_b}{K - \sum_{l=1}^{K} Z_{jl}}} (1 - \pi_{jk}^*)^{\sum_{l=1}^{K} Z_{jl}} \right\}.$$

The acceptance probability for a deactivation step is obtained from the same expression but with inverse ratio.

When we extend the model and introduce $\mathbf{Z}_j$ the posterior changes so that the sampling of the other variables has to be modified. As an example the conditional distribution of $\mathbf{\Psi}_k$ changes to

$$W\left(\left(\mathbf{H}_k + \sum_{h=1}^{J} Z_{hk}\mathbf{\Sigma}_{jk}^{-1}\right)^{-1},\ \nu^* + \nu_k\sum_{h=1}^{J} Z_{hk}\right).$$

We do not display all the changes since they are notationally complicated but otherwise straightforward, except for the label switching step. Suppose we propose to change $k_1$ to $k_2$ where $k_1$ is an inactive cluster. Then the acceptance probability (2) changes to

$$\alpha(k_1, k_2) = \min\left(1, \frac{\pi(\boldsymbol{\mu}_{jk_2}|\boldsymbol{\theta}_{k_1}, \mathbf{\Sigma}_{\theta_{k_1}})\pi(\mathbf{\Sigma}_{jk_2}|\mathbf{\Psi}_{k_1}, \nu_{k_1})}{\pi(\boldsymbol{\mu}_{jk_2}|\boldsymbol{\theta}_{k_2}, \mathbf{\Sigma}_{\mu_{k_2}})\pi(\mathbf{\Sigma}_{jk_2}|\mathbf{\Psi}_{k_2}, \nu_{k_2})}\right). \tag{4}$$

# C Merging latent clusters

The merging of latent clusters is done in a hierarchical fashion. In each step we have a number of latent super clusters comprising of one or more latent clusters. The corresponding super components in each sample are mixtures of Gaussians, a representation which is hard to work with. It is useful to instead use the data perspective, i.e. to consider the soft clustering of the data induced by the GMM of each sample.

For each sample we define super cluster $k$ from the probabilities for each of the data points in that sample to belong to any of the components linked to the latent super cluster $k$. We denote cluster $k$ in sample $j$ by $\Gamma_{k,j}$ =

$(\mathbf{Y}_{ij}, w_{ijk})_{i=1}^{n_j}$, where $w_{ijk}$ is the probability that $\mathbf{Y}_{ij}$ belongs to super cluster $k$. The parameter $w_{ijk}$ can be estimated from the sampling of $x_{ij}$.

To determine candidates for the subsequent merger, Bhattacharyya distance is computed between all pairs of current clusters in each sample. To do this we approximate each $\Gamma_{k,j}$ with a Gaussian distribution with parameters

$$\boldsymbol{\mu}^{(kj)} = \sum_{i=1}^{n_j} w_{ijk}\mathbf{Y}_{ij}, \qquad \boldsymbol{\Sigma}^{(kj)} = \sum_{i=1}^{n_j} w_{ijk}(\mathbf{Y}_{ij} - \boldsymbol{\mu}^{(kj)})(\mathbf{Y}_{ij} - \boldsymbol{\mu}^{(kj)})^\top$$

and use formula (4), so

$$d_{\text{bhat}}(\Gamma_{k,j}, \Gamma_{l,j}) = 1/8 \cdot (\boldsymbol{\mu}^{(kj)} - \boldsymbol{\mu}^{(lj)})^\top \bar{\boldsymbol{\Sigma}}^{-1}(\boldsymbol{\mu}^{(kj)} - \boldsymbol{\mu}^{(lj)}) + 1/2 \cdot \log\left(|\bar{\boldsymbol{\Sigma}}|/\sqrt{|\boldsymbol{\Sigma}^{(kj)}||\boldsymbol{\Sigma}^{(lj)}|}\right),$$

where $\bar{\boldsymbol{\Sigma}} = (\boldsymbol{\Sigma}^{(kj)} + \boldsymbol{\Sigma}^{(lj)})/2$. The candidates for the subsequent merger are the pair of clusters $(k, l)$—which among those pairs who have not previously been evaluated for merging—has highest median of $\exp(-d_{\text{bhat}}(\Gamma_{kj}, \Gamma_{lj}))$ across samples $j$. It is natural to consider $\exp(-d_{\text{bhat}})$ instead of $d_{\text{bhat}}$ when comparing Bhattacharyya distances since $\exp(-d_{\text{bhat}})$ is an upper bound of the misclassification probability between the components (Fukunaga, 1990).

If $\text{Med}_j(\exp(-d_{\text{bhat}}(\Gamma_{kj}, \Gamma_{lj}))) > h_1$, where $\text{Med}(\cdot)$ denotes the median, latent clusters $k$ and $l$ are immediately merged. On the other hand, if $h_1 > \text{Med}_j(\exp(-d_{\text{bhat}}(\Gamma_{kj}, \Gamma_{lj}))) > h_2$, they are merged only if the resulting cluster does not have sufficient evidence of being multimodal. Finally, if $\text{Med}_j(\exp(-d_{\text{bhat}}(\Gamma_{kj}, \Gamma_{lj}))) < h_2$ they are not merged and the procedure is stopped.

To evaluate multimodality of potential mergers we apply Hartigan's dip test of unimodality (Hartigan and Hartigan, 1985) to the projection of the merged cluster onto each coordinate axis and to the projection onto Fisher's discriminant coordinate separating the two clusters, namely $u = (\boldsymbol{\Sigma}^{(kj)} + \boldsymbol{\Sigma}^{lj})^{-1}(\boldsymbol{\mu}^{(kj)} - \boldsymbol{\mu}^{(lj)})$ (Fisher, 1936). Hartigan's dip statistic is computed from the empirical distribution function, which can readily be computed for these soft clusters from $(\mathbf{Y}_{ij}, w_{ijk})_{i=1}^{n_j}$. If for any of the projections, 25% of the samples or more get a $p$-value below the threshold $h_d$ we do not merge.

To determine the thresholds $h_1$, $h_2$ and $h_d$ we use results from two experiments performed by Hennig ((2010)). Synthetic data were generated from distributions which naturally represent a single cluster and a number of

Gaussian components were fitted to the data. For different criteria, threshold values for merging the components to one cluster in 95% of the cases, were then reported. The experiments were performed over a range of different dimensions and number of data points. We consider only results for distributions of dimension two to five and for at least 100 and at most 500 points, since for most of the flow cytometry samples in the data set studied in Section 3.2 a small cluster containing 1% of the data points would have about 200 data points.

In the first experiment two components were fitted to data generated from a unimodal mixture of two Gaussian distributions with the property that if the means were further apart the density would be bimodal. In the second experiment six Gaussian components were fitted to data generated from uniform distributions on hypercubes. The merging of the six components were made in a hierarchical procedure similar to ours.

When Bhattacharyya distance was used as merging criterion the threshold for $\exp(-d_{\text{bhat}})$ varied between 0.40 and 0.53 in the first experiment. For the second experiment we considered four combinations of dimension and number of data points and for these the thresholds were 0.12, 0.17, 0.01 and 0.11 respectively. This lead us to use $h_1 = 0.47$ as the soft threshold and $h_2 = 0.08$ as the soft threshold.

Hartigan's dip test was also evaluated as a criterion for merging, but only the first of the experiments is relevant for our use of it, since we only use the dip test to evaluate proposed mergers and not select candidates for merging. Only projections onto Fisher's discriminant coordinate were considered in the experiment. The threshold for the $p$-value varied between 0.15 and 0.41, so we chose $h_d = 0.28$. It should be noted that this cannot be translated into a significance level since the tests are done in a data-dependent way.

# D Simulation study

## D.1 Data generation

In this section the method for generating the simulated data is presented. The four latent means are

$$\boldsymbol{\theta}_1 = [0, 0, 0],\ \boldsymbol{\theta}_2 = [0, -2, 1],\ \boldsymbol{\theta}_3 = [1, 2, 0],\ \boldsymbol{\theta}_4 = [-2, 2, 1.5].$$

Each $\boldsymbol{\mu}_{jk}$ in the simulation is generated by

$$\begin{aligned}\boldsymbol{\mu}_{jk} &= \boldsymbol{\theta}_k + \mathbf{Z}_{jk},\ k = 1, 2, 3, 4\\ \mathbf{Z}_{jk} &\sim\ N(\mathbf{0}, \boldsymbol{\Sigma}_{\mu_k}),\end{aligned}$$

where

$$\boldsymbol{\Sigma}_{\mu_1} = \begin{bmatrix} 1.27 & 0.25 & 0 \\ 0.25 & 0.27 & -0.001 \\ 0 & -0.001 & 0.001 \end{bmatrix}, \qquad \boldsymbol{\Sigma}_{\mu_2} = \begin{bmatrix} 0.06 & 0.04 & -0.03 \\ 0.04 & 0.05 & 0 \\ -0.03 & 0. & 0.09 \end{bmatrix},$$

$$\boldsymbol{\Sigma}_{\mu_3} = \begin{bmatrix} 0.44 & 0.08 & 0.08 \\ 0.08 & 0.16 & 0 \\ 0.08 & 0 & 0.16 \end{bmatrix}, \qquad \boldsymbol{\Sigma}_{\mu_4} = 0.01\mathbf{I}.$$

The covariance matrices are generated through

$$\boldsymbol{\Sigma}_{jk} \sim IW((\nu_k - 3)\boldsymbol{\Psi}_k, \nu_k),\ k = 1, 2, 3, 4,$$

where

$$\boldsymbol{\Psi}_1 = 0.1\mathbf{I}, \qquad \boldsymbol{\Psi}_2 = 0.1 \begin{bmatrix} 2.0 & 0.5 & 0 \\ 0.5 & 2.0 & 0.5 \\ 0 & 0.5 & 2.0 \end{bmatrix},$$

$$\boldsymbol{\Psi}_3 = 0.1 \begin{bmatrix} 2.0 & -0.5 & 1.0 \\ -0.5 & 2.0 & -0.5 \\ 1.0 & -0.5 & 2.0 \end{bmatrix}, \qquad \boldsymbol{\Psi}_4 = 0.1 \begin{bmatrix} 1.0 & 0.3 & 0.3 \\ 0.3 & 1.0 & 0.3 \\ 0.3 & 0.3 & 1.0 \end{bmatrix},$$

and $\nu_k = 100$ for all $k$. Finally, $\boldsymbol{\pi}_j = [0.49, 0.3, 0.2, 0.01]$ if all clusters are present. If one or two clusters are not present the ratio of the probabilities for the present clusters remains the same.

## D.2 Priors

The priors are set to represent non informative priors; the priors are set equal for all classes. The exact values are:

$$\begin{aligned}\mathbf{S}_k &= 10^6\mathbf{I}_d, \mathbf{t}_k = \mathbf{0},\\ \mathbf{H}_k &= 10^{-6}\mathbf{I}_d, n_{\psi_k} = d,\\ \mathbf{Q}_k &= 10^{-6}\mathbf{I}_d, n_{\theta_k} = d,\\ l_k &= 0.01,\end{aligned}$$

for $t = 1, 2, 3, 4$.

## D.3 Initialization

Before running the MCMC sampler to get samples from the posterior distribution, we utilize the following initialization to get suitable initial parameter values. First we set all mean parameters $\boldsymbol{\mu}_{jk}$ and $\boldsymbol{\theta}_k$ to $\mathbf{0}$ and all covariance and precision matrices $\boldsymbol{\Sigma}_{jk}$, $\boldsymbol{\Sigma}_{\theta_k}$ and $\boldsymbol{\Psi}_k$ to $\mathbf{I}$. Then after letting the MCMC sampler run for 5000 iterations, without the option of turning off components, we link all the components across samples through the following procedure:

1. The first sample is left unchanged.

2. For the second sample the components are first sorted by $\boldsymbol{\pi}_2$, so we get ordered components $(\boldsymbol{\mu}_{2(i)}, \boldsymbol{\Sigma}_{2(i)}, \pi_{2(i)})$ for $i = 1, 2, 3, 4$, where $\pi_{2(1)} \geq \pi_{2(2)} \geq \pi_{2(3)} \geq \pi_{2(4)}$. Then the first component $(\boldsymbol{\mu}_{2(1)}, \boldsymbol{\Sigma}_{2(1)}, \pi_{2(1)})$ is matched to the component $k$ whose mean $\boldsymbol{\mu}_{1k}$ is closest to $\boldsymbol{\mu}_{2(1)}$. If for example we have that $\boldsymbol{\mu}_{13}$ is closest to $\boldsymbol{\mu}_{2(1)}$ we set $(\boldsymbol{\mu}_{23}, \boldsymbol{\Sigma}_{23}, \pi_{23}) = (\boldsymbol{\mu}_{2(1)}, \boldsymbol{\Sigma}_{2(1)}, \pi_{2(1)})$. This is repeated for $(\boldsymbol{\mu}_{2(i)}, \boldsymbol{\Sigma}_{2(i)}, \pi_{2(i)})$, $i = 2, 3, 4$, but indices which have already been assigned to components are excluded from consideration.

3. For the remaining samples we proceed as for the second sample, with the exception that the matching of $\boldsymbol{\mu}_{j(k)}$ is now done to the average of the $j-1$ previously matched clusters means, namely $(j-1)^{-1}\sum_{l=1}^{j-1}\boldsymbol{\mu}_{lk}$ for $k = 1, 2, 3, 4$.

# E Flow cytometry data analysis

## E.1 Data set details

Antibodies against CD45, CD19, CD3, CD8 and CD4 linked to fluorochromes were used to mark the PBMC and when passed through the flow cytometer the expression of these markers were measured along with front and side scatter. A standard transformation called compensation was used to remove effects of spectral overlap (Azad et al., 2013). Following this the data was transformed using the function $\operatorname{asinh}(y/c)$, where $c$ was chosen to minimize Bartlett's statistic, with the purpose to stabilize variance between markers. Measurements corresponding to lymphocytes were selected using front and side scatter by fitting a bivariate normal distribution and filtering based on a likelihood threshold using the norm2Filter function in the flowCore R

package (Azad, personal communication). This resulted in between 6172 and 19,554 cell measurements for each sample. Since all lymphocytes are CD45+, only the other four markers were retained. We loaded this data from the R package healthyFlowData and scaled it using the 1% and 99% percentiles $q_{0.01}$ and $q_{0.99}$ of the pooled data, with the same scaling for all samples, so that $q_{0.01} = 0$ and $q_{0.99} = 1$ for each marker for the pooled data.

## E.2 Prior parameters and initialization

Using our first piece of prior information, we set $t_{mk}$ to 0.15 if population $k$ is negative for marker $m$, 0.85 if population $k$ is positive for marker $m$ and 0.5 otherwise. To model the uncertainty in latent cluster locations we let $\mathbf{S}_k = \text{diag}(\sigma_{1k}^2, \sigma_{2k}^2, \sigma_{3k}^2, \sigma_{4k}^2)$, where $\sigma_{mk}$ is 0.05 if the population is positive or negative for marker $m$ and 100 otherwise. For the remaining latent components we set non-informative priors on cluster locations, i.e. $t_{mk} = 0.5$ for all dimensions $m$ and $\mathbf{S}_k = 10^6 \cdot \text{Var}(\mathbf{Y})$, where $\mathbf{Y}$ is the pooled data.

For the parameters $\mathbf{Q}_k$, $n_{\theta_k}$ and $n_{\Psi_k}$ our second piece of prior information leads us to choose values leading to as non-informative priors as possible, while still being restrictive enough to make the latent clusters amenable to biological interpretation. The parameter values we use are $n_{\theta_k} = 1000$, $\mathbf{Q}_k = (n_{\theta_k} - d - 1) \cdot 10^{-4}\mathbf{I}$ and $n_{\Psi_k} = 50$. The parameter $\mathbf{H}_k$ is chosen to give an expected value of the latent covariance matrices which is slightly larger than what we expect to see in the data, which gives fast convergence. We choose $\mathbf{H}_k = (1/3)^2 n_{\Psi_k}/(n_{\Psi_k} - d - 1) \cdot \mathbf{I}$, which implies that the expected value of each $\mathbf{\Sigma}_{\theta_k}$ is $10^{-4}\mathbf{I}$ and that if $\nu_k = n_{\Psi_k}$ the expected value of each $\mathbf{\Psi}_k$ is $(1/3)^2\mathbf{I}$.

Initialization of the variables $\boldsymbol{\mu}_{jk}, \boldsymbol{\theta}_k, \mathbf{\Sigma}_{\theta_k}, \mathbf{\Sigma}_{jk}, \mathbf{\Psi}_k, \boldsymbol{\pi}_j$ for the known populations is done by setting them to the expected values of their priors given that the other variables have the expected values of their respective priors and that $\nu_k = n_{\Psi_k}$. For each unknown population we use the same procedure except that $\theta_{mk}$ is drawn from $N(t_{mk}, 0.3^2)$, $m = 1, \ldots, 4$.

During the burn-in period, in each iteration we select a pair of components in each sample with probability 0.1 to propose for label switch. We do not utilize the possibility to turn on and off clusters for this data set, and thus set $p_a = p_d = 0$.

## E.3 Additional results

### E.3.1 Convergence

We assess the convergence of the MCMC sampler by looking at trace plots for $\boldsymbol{\theta}_k$ and $\nu_k$, where $k \in \{1, \ldots, K\}$. These are shown in Fig. 1 and Fig. 2. Convergence is obtained after typically 10,000 iterations.

### E.3.2 Marginal distributions

To evaluate the similarity between one- and two-dimensional marginal distributions of the model of the data, for each production iteration we generate one synthetic data point from the GMM of two different flow cytometry samples—sample 3 and sample 6—and from the model of the pooled data. The one- and two-dimensional histograms of sample 6 are shown in the main article, Fig. 8, the one- and two-dimensional histograms of sample 3 are shown in Fig. 3. The one- and two-dimensional histograms of samples from the model of the pooled data are shown in Fig. 4. The synthetic data agrees well with the real data for both the two samples and for the pooled data.

### E.3.3 Unimodality

We want to detect if the distribution of data assigned to a single component or super component is not unimodal, since it indicates that the latent cluster maybe should be divided into two or more components. To do this we use Hartigan's dip test (Hartigan and Hartigan, 1985) of unimodality for the one-dimensional marginal distributions.

Results are plotted in Fig. 5. Even though the single components frequently have multimodal distributions for the data assigned to them, for the super components the lower quartiles are well above the threshold below which we consider the clusters multimodal in the merging procedure ($h_d = 0.28$). This is even the case for the minimum—except for the smallest cluster with NK-like cells.

### E.3.4 Unknown population

In the analysis of the real flow cytometry data set, one population was found which was not specified in the priors. This population does also fit the criteria in Table 1 for NK cells, but there are strong evidence that it is a

separate population. Fig. 6 show histograms of CD4 measurements in the new population and the original NK population for the twenty flow cytometry samples. In most of the samples, the populations are well separated.

# References


A. Azad, A. Khan, B. Rajwa, S. Pyne, and A. Pothen. Classifying immunophenotypes with templates from flow cytometry. In Proceedings of the International Conference on Bioinformatics, Computational Biology and Biomedical Informatics, page 256. ACM, 2013.

R. A. Fisher. The use of multiple measurements in taxonomic problems. Annals of eugenics, 7(2):179–188, 1936.

K. Fukunaga. Introduction to Statistical Pattern Recognition. Academic press, 1990.

P. J. Green. Reversible jump markov chain monte carlo computation and bayesian model determination. Biometrika, 82(4):711–732, 1995. doi: 10.1093/biomet/82.4.711. URL `http://biomet.oxfordjournals.org/content/82/4/711.abstract`.

J. A. Hartigan and P. M. Hartigan. The dip test of unimodality. The Annals of Statistics, pages 70–84, 1985.

C. Hennig. Methods for merging Gaussian mixture components. Advances in Data Analysis and Classification, 4(1):3–34, 2010.

S. Richardson and P. J. Green. On Bayesian analysis of mixtures with an unknown number of components (with discussion). Journal of the Royal Statistical Society: Series B (Statistical Methodology), 59(4):731–792, 1997. ISSN 1467-9868. doi: 10.1111/1467-9868.00095. URL `http://dx.doi.org/10.1111/1467-9868.00095`.

C. Robert and G. Casella. Monte Carlo Statistical Methods. Springer Texts in Statistics. Springer, 2004. ISBN 9780387212395.

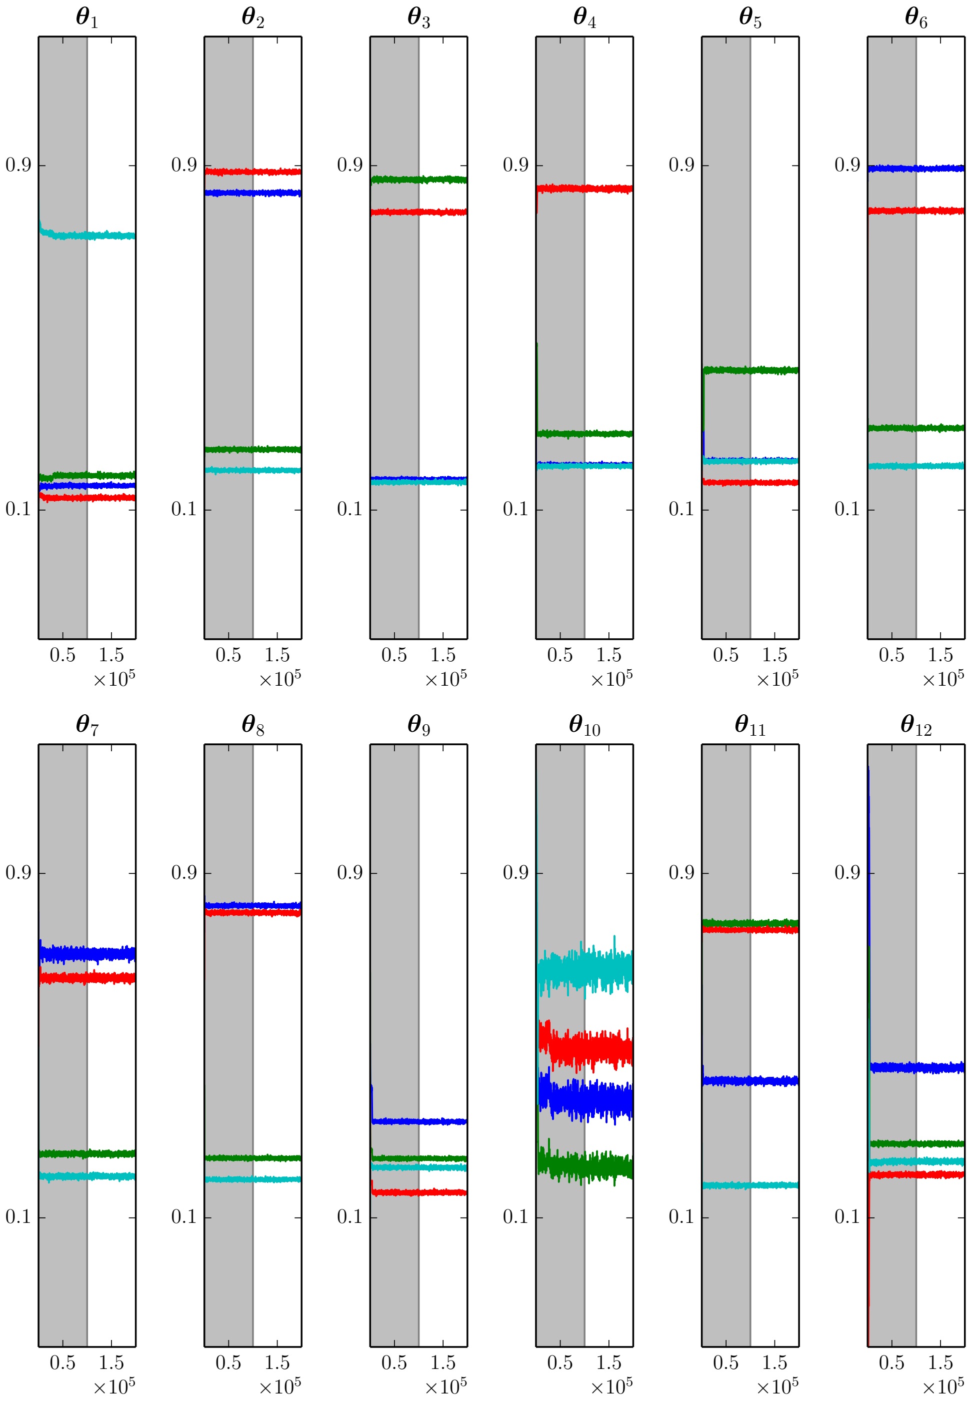


Figure 1: Trace plots of latent means $\theta_k$ for $k = 1, \ldots, 12$ for experiment described in Section 3.2. Burn-in iterations are plotted on grey background.

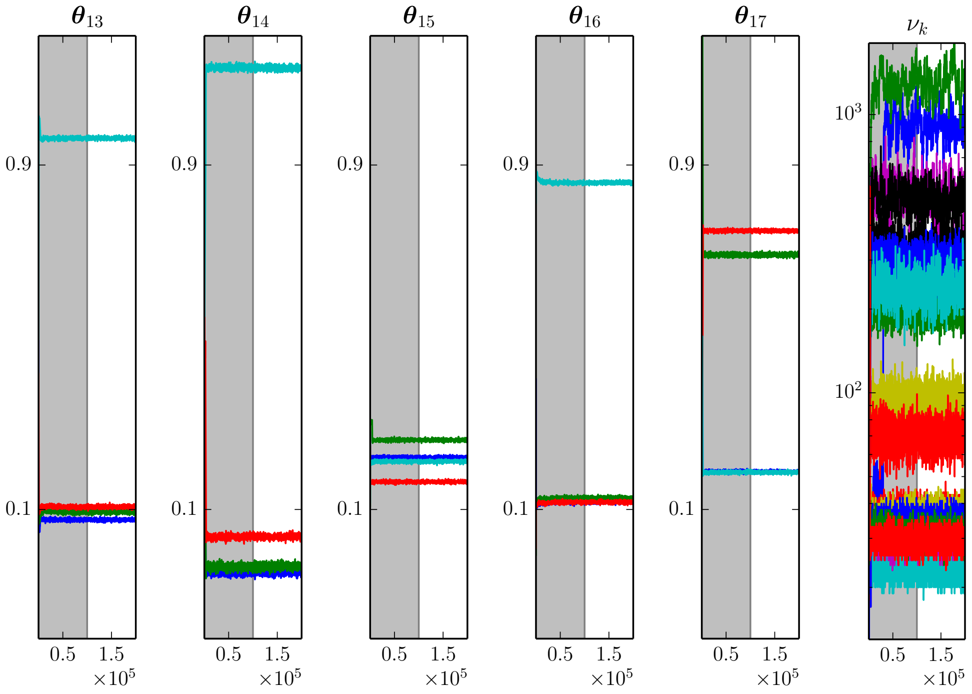


Figure 2: Trace plots of latent means $\theta_k$ for $k = 13, \ldots, 17$ and parameters $\nu_k$ for $k = 1, \ldots, 17$ for experiment described in Section 3.2. Burn-in iterations are plotted on grey background.

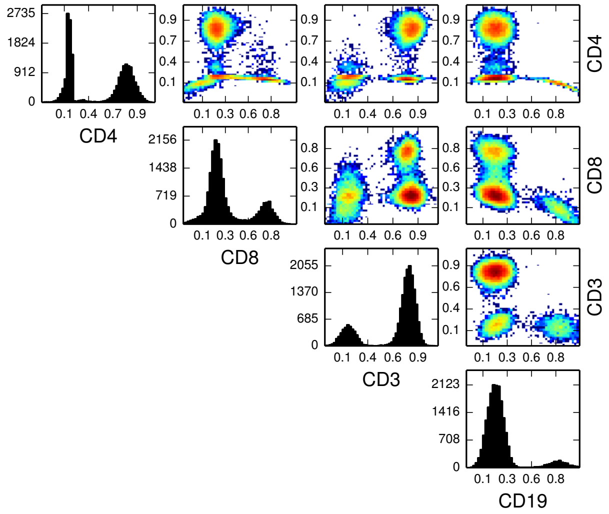


(a)

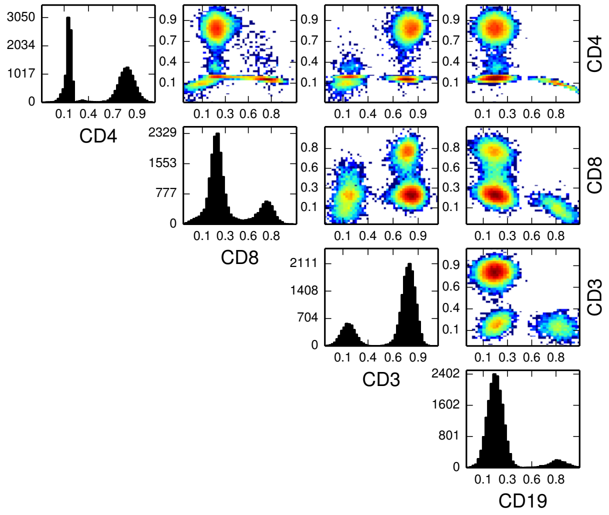


(b)

Figure 3: One and two dimensional histograms of flow cytometry data. (a) One of the samples from healthyFlowData, with 19,138 data points. (b) 19,138 data points drawn from the inferred model of the sample.

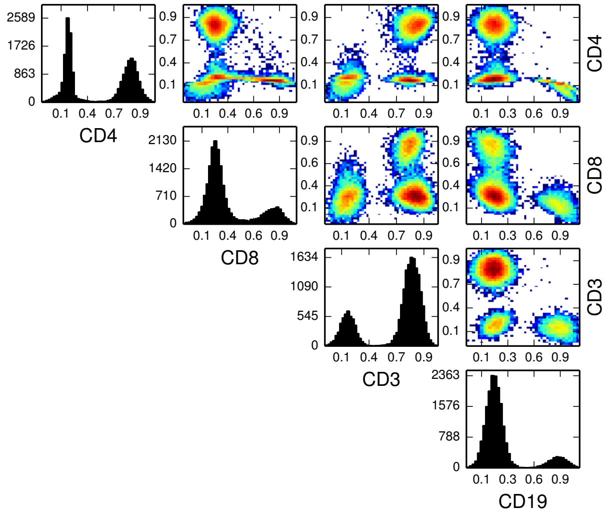


Figure 4: One and two dimensional histograms of samples drawn from model of flow cytometry data. 19,160 data points drawn from the model of twenty samples in healthyFlowData pooled together. The pooled data is quite different from the single sample and seem to have a much more complex density.

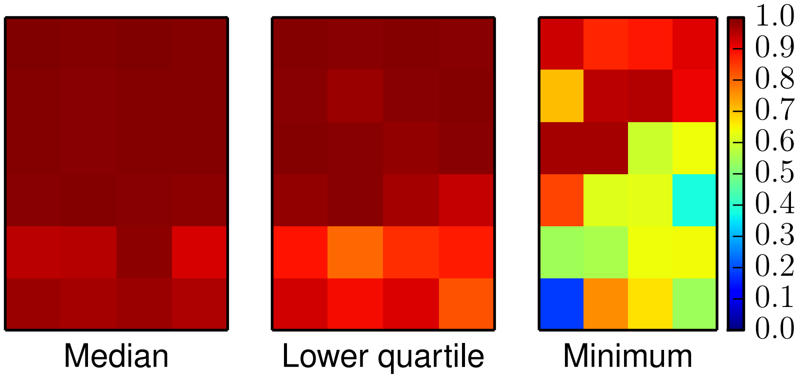


(a)

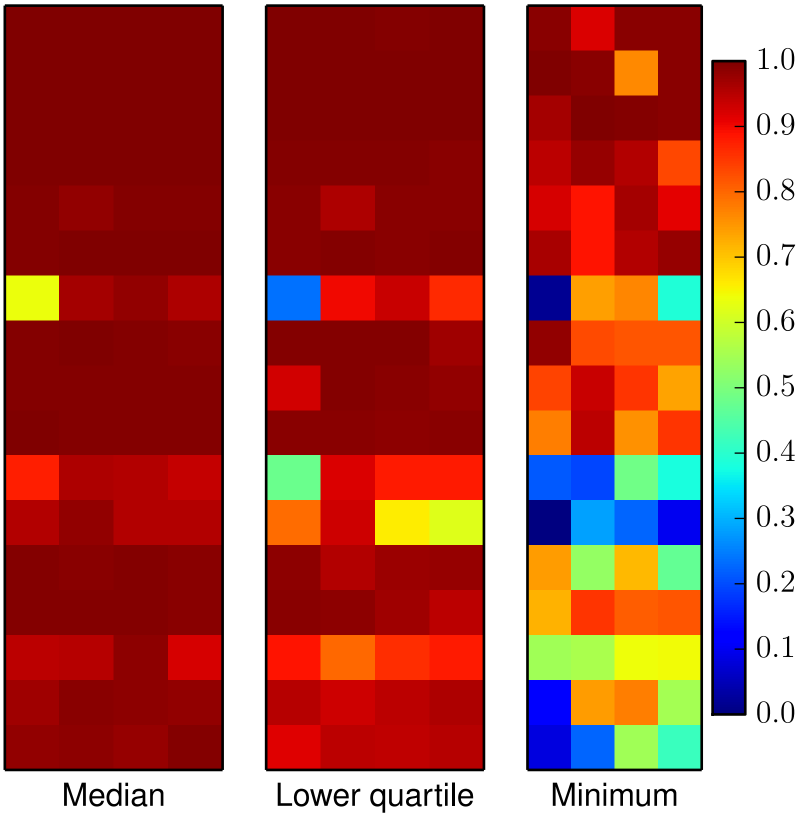


(b)

Figure 5: Median, lower quartile and minimum—taken across flow cytometry samples—for $p$-values of dip tests of unimodality. In each matrix the first column is along the CD4 dimension, the second is along the CD8 dimension, the third along the CD3 dimension and the fourth along the CD19 dimension. The rows are ordered by estimated mixture proportions $\hat{\pi}_{jk}$, with highest first. (a) Merged clusters. (b) Original clusters, before merging.

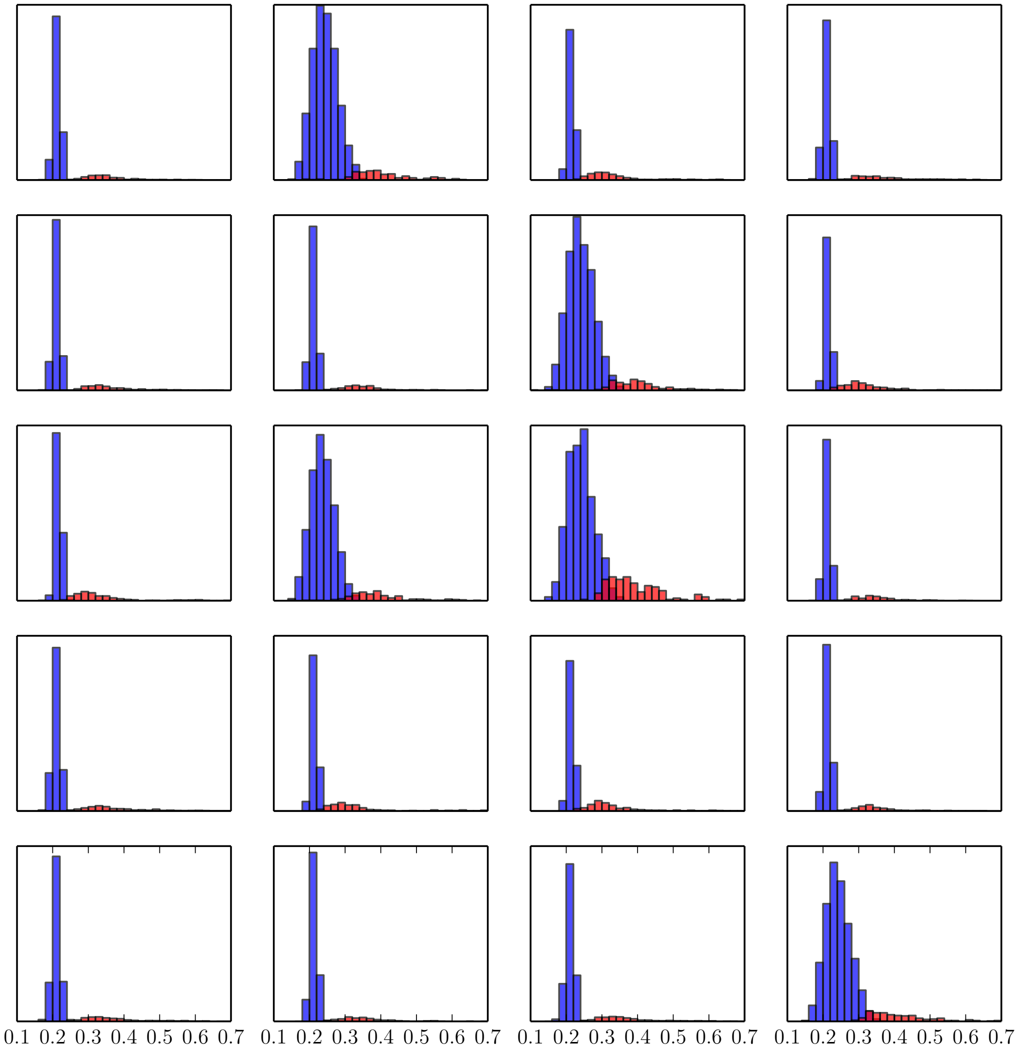


Figure 6: Histograms of CD4 expression of cells with more than 30% posterior probability of belonging to the NK cell population (blue) or the $CD4^{dim}CD3-$ CD19– population (red). Each histogram depicts results for one flow cytometry sample.
